# Supplementary material for: XR Prototyping of Mixed Reality Visualizations: Compensating Interaction Latency for a Medical Imaging Robot
Source: arXiv:2409.04900 source file (2024-09-16)
Supplement: Supplementary file 1 [file 09_appendix.tex]

\newpage
\section{Appendix}
\begin{figure*}[]
    \centering
    \includegraphics[width=\textwidth]{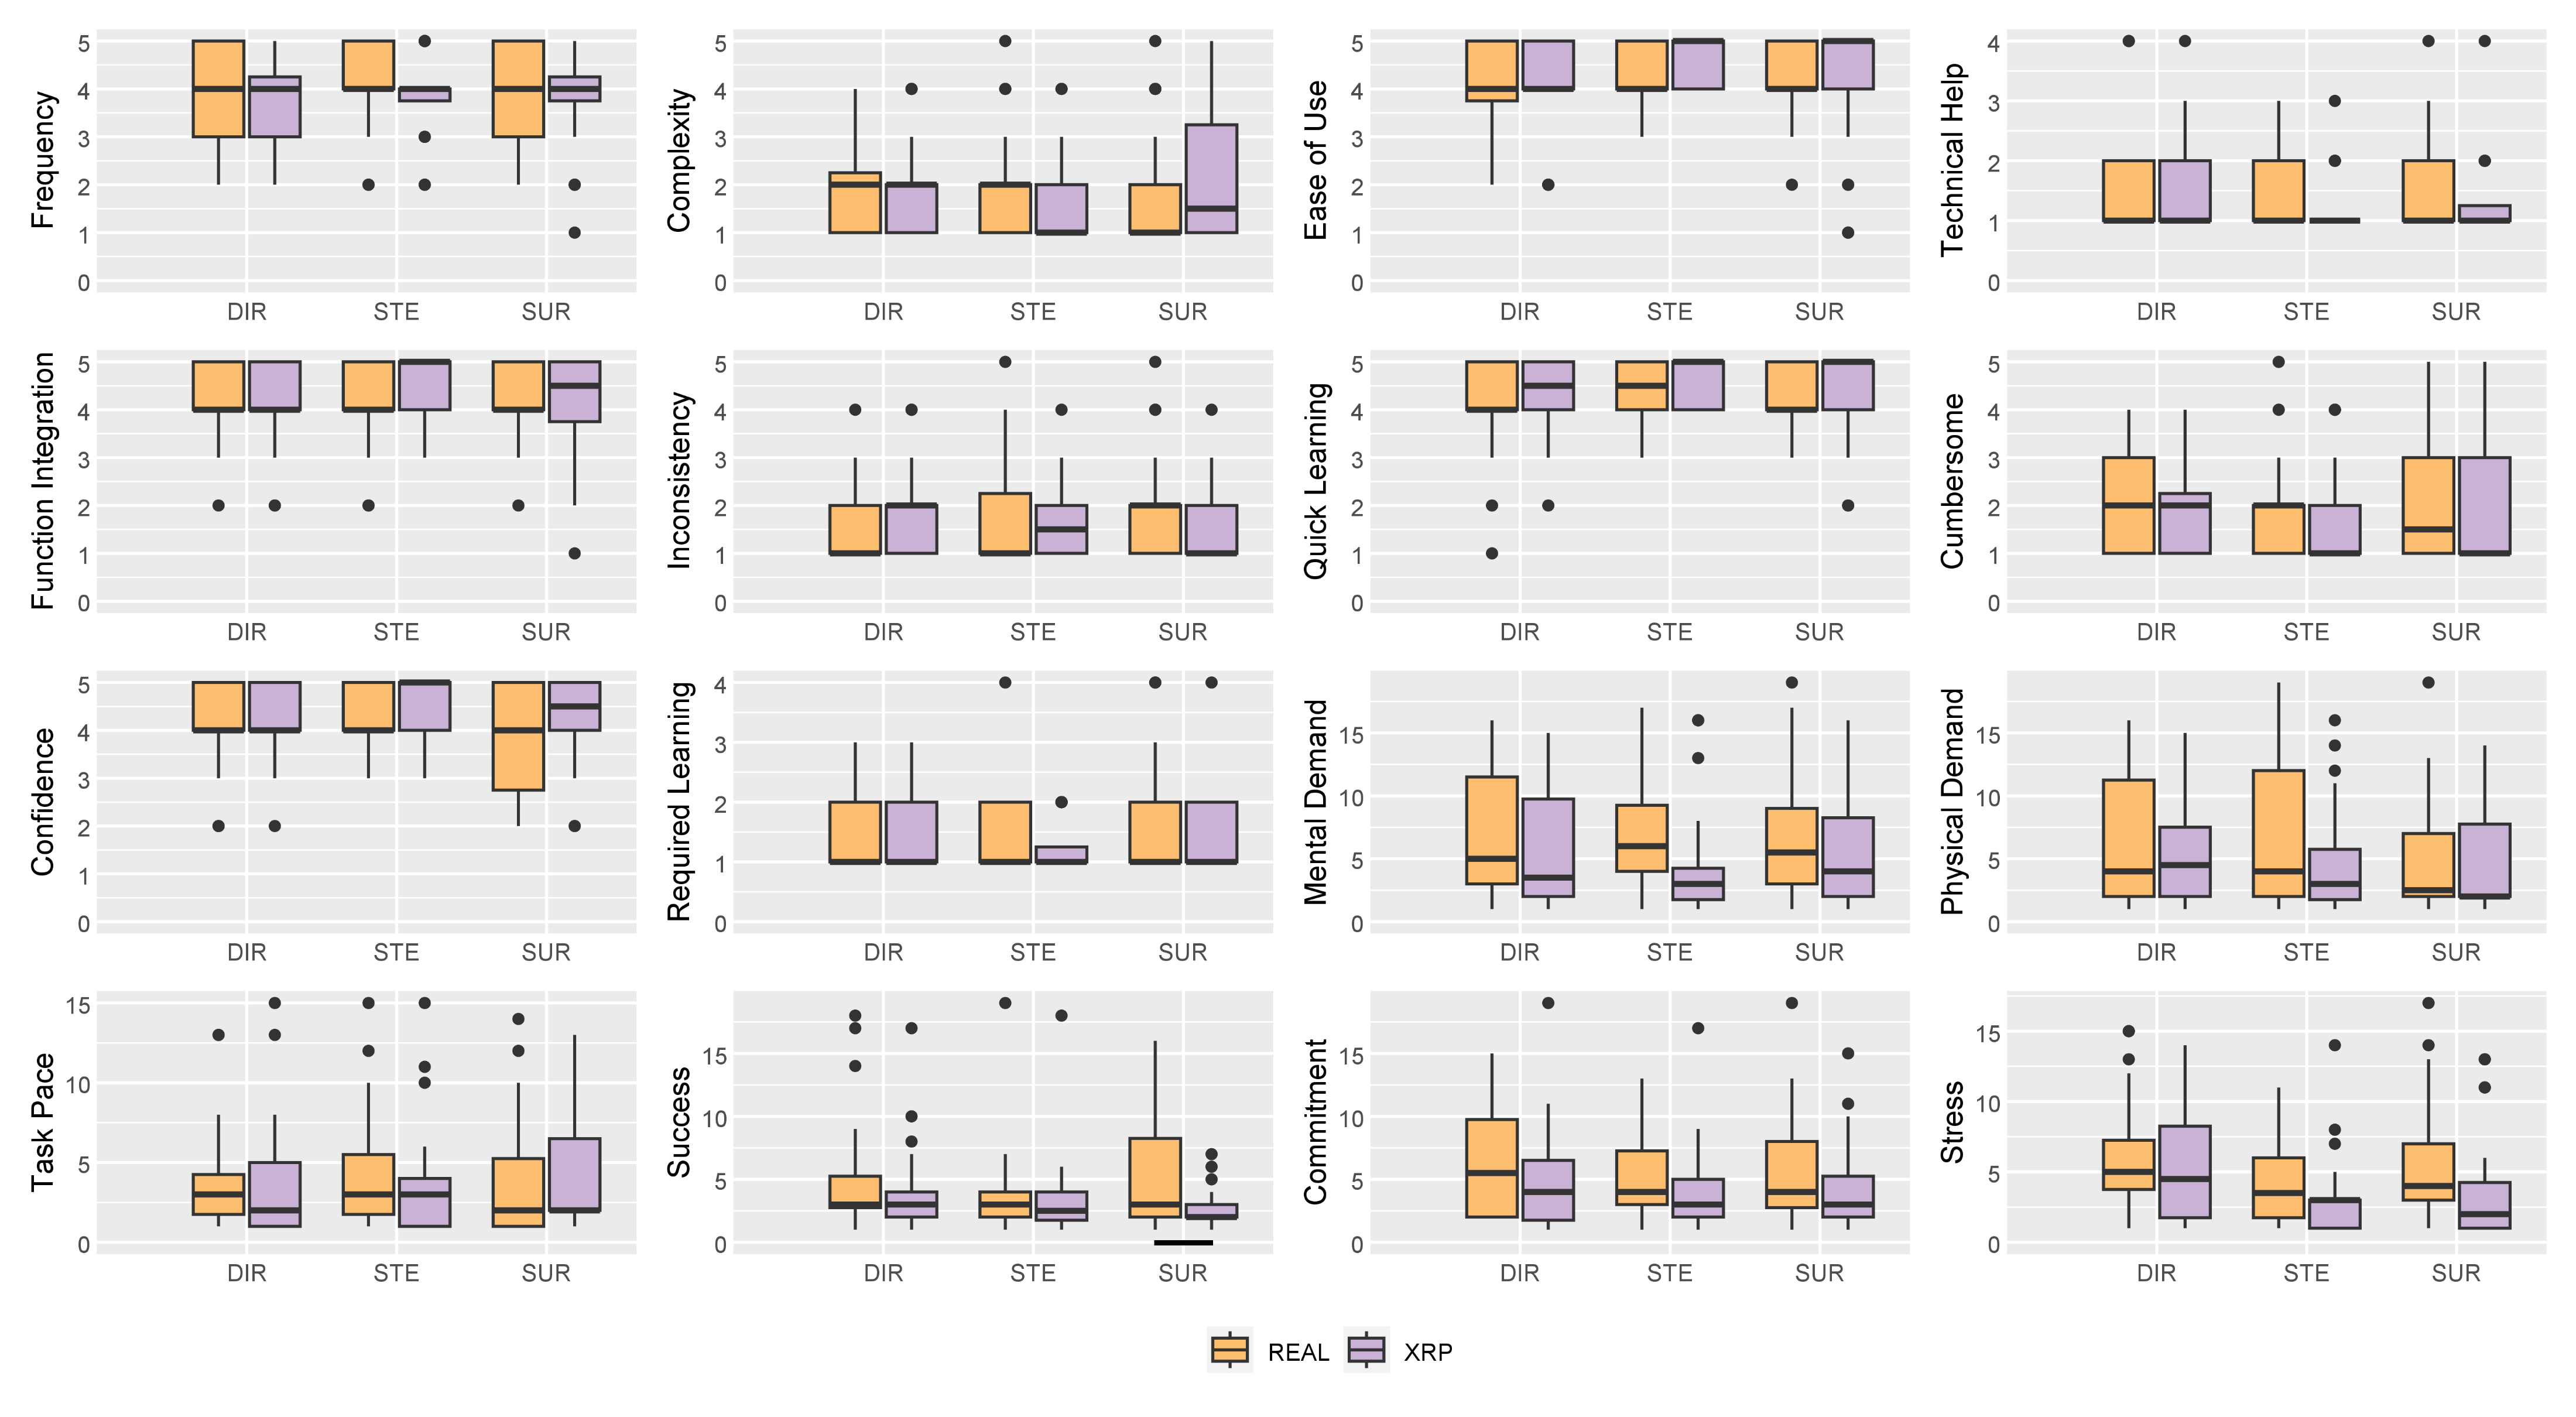}
    \caption{
        Box plots of individual Realism and Visualization combinations. Statistically significant differences are marked.
    }
    \label{fig:combined_conditions}
\end{figure*}
\begin{table*}[!t]
    \scriptsize
    \begin{tabularx}{\textwidth}{l||X|X|X||X|X|X}
        & \multicolumn{3}{c||}{\condREAL{}} & \multicolumn{3}{c}{\condXRP{}} \\
        \hline
        & \condDIR{} & \condSTE{} & \condSUR{} & \condDIR{} & \condSTE{} & \condSUR{} \\    
        \hline
        \hline
        TCT & \data{135.25}{47.72}{115.0} & \data{133.06}{31.08}{131.8} & \data{86.25}{89.72}{46.6} & \data{111.33}{31.83}{108.6} & \data{112.54}{30.18}{115.9} & \data{66.85}{40.04}{49.5} \\ 
        \hline
        \hline
        Frequency & \data{3.75}{1.03}{4.0} & \data{4.04}{1.00}{4.0} & \data{3.79}{1.18}{4.0} & \data{3.75}{1.03}{4.0} & \data{3.83}{0.92}{4.0} & \data{3.75}{1.15}{4.0} \\

        Complexity & \data{2.00}{1.10}{2.0} & \data{1.88}{1.12}{2.0} & \data{1.88}{1.23}{1.0} & \data{1.92}{1.02}{2.0} & \data{1.50}{0.93}{1.0} & \data{2.08}{1.35}{1.5} \\
        
        Ease of Use & \data{4.00}{0.93}{4.0} & \data{4.38}{0.58}{4.0} & \data{4.21}{0.88}{4.0} & \data{4.08}{1.06}{4.0} & \data{4.58}{0.50}{5.0} & \data{4.12}{1.33}{5.0} \\
        
        Technical Help & \data{1.58}{0.88}{1.0} & \data{1.50}{0.66}{1.0} & \data{1.54}{0.83}{1.0} & \data{1.46}{0.83}{1.0} & \data{1.25}{0.53}{1.0} & \data{1.33}{0.70}{1.0} \\
        
        Function Integration & \data{4.21}{0.88}{4.0} & \data{4.08}{0.93}{4.0} & \data{4.17}{0.87}{4.0} & \data{4.04}{0.86}{4.0} & \data{4.46}{0.66}{5.0} & \data{4.04}{1.23}{4.5} \\
        
        Inconsistency & \data{1.62}{0.88}{1.0} & \data{1.88}{1.19}{1.0} & \data{1.88}{1.12}{2.0} & \data{1.83}{0.96}{2.0} & \data{1.67}{0.82}{1.5} & \data{1.54}{0.88}{1.0} \\
        
        Quick Learning & \data{4.12}{0.99}{4.0} & \data{4.46}{0.59}{4.5} & \data{4.33}{0.64}{4.0} & \data{4.38}{0.77}{4.5} & \data{4.58}{0.50}{5.0} & \data{4.33}{0.96}{5.0} \\
        
        Cumbersome & \data{2.17}{1.09}{2.0} & \data{1.88}{1.08}{2.0} & \data{2.00}{1.25}{1.5} & \data{2.04}{1.00}{2.0} & \data{1.75}{1.03}{1.0} & \data{2.04}{1.33}{1.0} \\
        
        Confidence & \data{4.21}{0.88}{4.0} & \data{4.29}{0.69}{4.0} & \data{3.88}{1.26}{4.0} & \data{4.21}{0.83}{4.0} & \data{4.58}{0.58}{5.0} & \data{4.25}{0.94}{4.5} \\
        
        Required Learning & \data{1.42}{0.58}{1.0} & \data{1.46}{0.72}{1.0} & \data{1.54}{0.93}{1.0} & \data{1.46}{0.59}{1.0} & \data{1.25}{0.44}{1.0} & \data{1.38}{0.71}{1.0} \\

        \hline\hline
        
        Mental Demand & \data{7.00}{4.70}{5.0} & \data{6.88}{4.26}{6.0} & \data{6.58}{5.07}{5.5} & \data{5.79}{4.83}{3.5} & \data{4.54}{4.46}{3.0} & \data{5.58}{4.61}{4.0} \\

        Physical Demand & \data{6.46}{5.18}{4.0} & \data{6.33}{5.43}{4.0} & \data{5.04}{4.87}{2.5} & \data{5.17}{4.22}{4.5} & \data{4.67}{4.46}{3.0} & \data{4.96}{4.71}{2.0} \\
        
        Task Pace & \data{3.83}{3.41}{3.0} & \data{4.25}{3.85}{3.0} & \data{3.96}{3.75}{2.0} & \data{3.75}{3.79}{2.0} & \data{3.71}{3.59}{3.0} & \data{4.21}{3.73}{2.0} \\
        
        Success & \data{5.04}{4.75}{3.0} & \data{3.67}{3.60}{3.0} & \data{5.42}{4.45}{3.0} & \data{4.04}{3.54}{3.0} & \data{3.29}{3.44}{2.5} & \data{2.67}{1.55}{2.0} \\
        
        Commitment & \data{6.71}{4.61}{5.5} & \data{5.71}{4.03}{4.0} & \data{5.75}{4.52}{4.0} & \data{5.04}{4.27}{4.0} & \data{3.96}{3.28}{3.0} & \data{4.42}{3.74}{3.0} \\
        
        Stress & \data{6.00}{4.13}{5.0} & \data{4.46}{3.55}{3.5} & \data{5.67}{4.37}{4.0} & \data{5.29}{3.87}{4.5} & \data{3.08}{3.01}{3.0} & \data{3.71}{4.04}{2.0} \\

        \hline\hline
        
        Usability & \data{78.75}{15.97}{80.0} & \data{81.67}{12.28}{82.5} & \data{78.85}{19.01}{82.5} & \data{79.38}{15.06}{80.0} & \data{86.56}{10.60}{88.8} & \data{80.31}{19.59}{85.0} \\
        
        Task Load & \data{29.20}{18.18}{24.2} & \data{26.08}{15.45}{20.4} & \data{27.01}{18.16}{21.2} & \data{24.24}{15.08}{22.5} & \data{19.38}{14.30}{16.2} & \data{21.28}{14.69}{15.0} \\
    \end{tabularx}    
    \caption{Dependent variable outcomes (mean, std. dev., median) for each individual Realism and Visualization combination.}
    \label{tab:descriptive_fidelity_statistics}
\end{table*}
\begin{table*}[!t]
   \scriptsize
     \begin{tabularx}{\textwidth}{l||X|X|X||X|X}
        & \condDIR{} & \condSTE{} & \condSUR{} & \condREAL{} & \condXRP{} \\    
        \hline
        \hline
        TCT & \data{123.29}{41.91}{112.3} & \data{122.80}{32.03}{119.8} & \data{76.55}{69.42}{47.8} & \data{118.19}{64.62}{112.0} & \data{96.91}{40.01}{94.3} \\
        \hline
        \hline
        Frequency & \data{3.75}{1.02}{4.0} & \data{3.94}{0.95}{4.0} & \data{3.77}{1.15}{4.0} & \data{3.86}{1.07}{4.0} & \data{3.78}{1.02}{4.0} \\

        Complexity & \data{1.96}{1.05}{2.0} & \data{1.69}{1.03}{1.0} & \data{1.98}{1.28}{1.0} & \data{1.92}{1.14}{2.0} & \data{1.83}{1.13}{1.0} \\
        
        Ease of Use & \data{4.04}{0.99}{4.0} & \data{4.48}{0.55}{4.5} & \data{4.17}{1.12}{5.0} & \data{4.19}{0.82}{4.0} & \data{4.26}{1.03}{5.0} \\
        
        Technical Help & \data{1.52}{0.85}{1.0} & \data{1.38}{0.61}{1.0} & \data{1.44}{0.77}{1.0} & \data{1.54}{0.79}{1.0} & \data{1.35}{0.70}{1.0} \\
        
        Function Integration & \data{4.12}{0.87}{4.0} & \data{4.27}{0.82}{4.0} & \data{4.10}{1.06}{4.0} & \data{4.15}{0.88}{4.0} & \data{4.18}{0.95}{4.0} \\
        
        Inconsistency & \data{1.73}{0.92}{1.0} & \data{1.77}{1.02}{1.0} & \data{1.71}{1.01}{1.0} & \data{1.79}{1.06}{1.0} & \data{1.68}{0.89}{1.0} \\
        
        Quick Learning & \data{4.25}{0.89}{4.0} & \data{4.52}{0.55}{5.0} & \data{4.33}{0.81}{4.5} & \data{4.31}{0.76}{4.0} & \data{4.43}{0.77}{5.0} \\
        
        Cumbersome & \data{2.10}{1.04}{2.0} & \data{1.81}{1.04}{1.5} & \data{2.02}{1.28}{1.0} & \data{2.01}{1.13}{2.0} & \data{1.94}{1.12}{2.0} \\
        
        Confidence & \data{4.21}{0.85}{4.0} & \data{4.44}{0.65}{5.0} & \data{4.06}{1.12}{4.0} & \data{4.12}{0.98}{4.0} & \data{4.35}{0.81}{5.0} \\
        
        Required Learning & \data{1.44}{0.58}{1.0} & \data{1.35}{0.60}{1.0} & \data{1.46}{0.82}{1.0} & \data{1.47}{0.75}{1.0} & \data{1.36}{0.59}{1.0} \\
        \hline
        \hline
        
        Mental Demand & \data{6.40}{4.75}{4.0} & \data{5.71}{4.47}{4.0} & \data{6.08}{4.82}{4.5} & \data{6.82}{4.62}{5.0} & \data{5.31}{4.60}{3.5} \\

        Physical Demand & \data{5.81}{4.72}{4.0} & \data{5.50}{4.99}{3.0} & \data{5.00}{4.74}{2.0} & \data{5.94}{5.13}{3.5} & \data{4.93}{4.41}{3.0} \\
        
        Task Pace & \data{3.79}{3.57}{3.0} & \data{3.98}{3.69}{3.0} & \data{4.08}{3.70}{2.0} & \data{4.01}{3.63}{3.0} & \data{3.89}{3.66}{2.0} \\
        
        Success & \data{4.54}{4.18}{3.0} & \data{3.48}{3.49}{3.0} & \data{4.04}{3.58}{3.0} & \data{4.71}{4.30}{3.0} & \data{3.33}{3.00}{3.0} \\
        
        Commitment & \data{5.88}{4.48}{4.5} & \data{4.83}{3.74}{3.5} & \data{5.08}{4.16}{3.0} & \data{6.06}{4.36}{4.0} & \data{4.47}{3.76}{3.0} \\
        
        Stress & \data{5.65}{3.98}{5.0} & \data{3.77}{3.33}{3.0} & \data{4.69}{4.28}{3.0} & \data{5.38}{4.03}{4.0} & \data{4.03}{3.73}{3.0} \\
        \hline
        \hline
    
        Usability & \data{79.06}{15.36}{80.0} & \data{84.11}{11.62}{82.5} & \data{79.58}{19.11}{82.5} & \data{79.76}{15.82}{82.5} & \data{82.08}{15.64}{82.5} \\
    
        Task Load & \data{26.72}{16.71}{23.8} & \data{22.73}{15.11}{17.1} & \data{24.15}{16.60}{18.8} & \data{27.43}{17.11}{21.2} & \data{21.63}{14.63}{16.7} \\
    \end{tabularx}    
    \caption{Dependent variable outcomes (mean, std. dev., median) for each overall Realism and Visualization.}
    \label{tab:descriptive_statistics}
\end{table*}
